# Supplementary material for: Ion channels in critical membranes: clustering, cooperativity, and memory effects
Source: arXiv:2401.07660 ancillary file (2024-01-22)
Supplement: Supplementary file 1 [file Suppl_Mat.pdf]

# Supplemental Material – Ion channels in critical membranes: clustering, cooperativity, and memory effects

Antonio Suma,[1,2] Daniel Sigg,[2,3] Seamus Gallagher,[2] Giuseppe Gonnella,[1] and Vincenzo Carnevale[2]

[1]*Dipartimento di Fisica, Università degli Studi di Bari and INFN, Sezione di Bari, via Amendola 173, Bari, I-70126, Italy*

[2]*Institute for Computational Molecular Science, Temple University, Philadelphia, PA 19122, USA*

[3]*dPET, Spokane, WA, USA*

## I. DISTRIBUTION OF CLUSTERS OF ION CHANNELS FROM EXPERIMENTAL DATA

The authors of Ref. [1] provided us with a lists of observed individual cluster sizes gathered experimentally using super resolution microscopy. We then binned these data using a logarithmic scale, and computed the cluster size distributions (Fig. S1) for $Ca_v$ channels in Hippocampal neurons and tsA-201 cells.

The dotted line, referring to tsA-201 cells, is a fit done using a sum of two exponential distributions, $ae^{-x/b} + ce^{-x/d}$, with $a = 7.062 \cdot 10^{-4}, b = 1.473 \cdot 10^3, c = 2.217 \cdot 10^{-5}, d = 4.553 \cdot 10^3$. The dash-dotted line, referring to Hippocampal neurons, is a power law $ax^{-2.0549}$, with $a = 10^3$. The chosen exponent, as explained in the main text, is connected to the Fisher exponent $\tau = \frac{187}{91}$ of the 2D percolation transition [2].

We tested that the power law distribution is a reasonable hypothesis for the experimental distribution of Hippocampal neurons data using the procedure set out in Ref. [3]. Briefly, the test consists in using two estimators, described in the article, to compute the lower bound of the power-law behavior and the exponent, which for the distribution we considered are 3650 and 2.240, respectively. We then generated a large number of power-law distributed synthetic data sets, using the same exponent and lower bound as those estimated. The Kolmogorov-Smirnov (KS) statistics between the experimental data and the hypothesized power law was calculated, and compared to the one of synthetic data. The fraction of the time that the resulting statistic is larger than the value for the empirical data gives then a $p$-value. We found that $p = 0.056$, which supports the hypothesis.

Note that physically the power law distribution is a scale invariant feature that should not be observable at scales compatible with dimension of a single channel. Indeed, we see for the Hippocampal neurons that the distribution deviates from a power law at around 100nm$^2$, which is a size compatible with that of a single channel. Regarding instead the differences in distributions between different channels, arguably these depend on the environment and the channel expression within a cell.

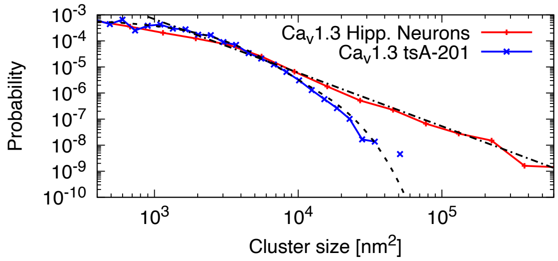


FIG. S1. Cluster size distribution of $Ca_v$ channels in Hippocampal neurons and tsA-201 cells. See text for details.

## II. MESOSCOPIC SIMULATIONS

A dumbbell, representing a lipid type, consists of a pair of particles with one bead (type 1 particle) constrained to move on the plane $z = 0$, while the second bead (type 2 particle) is connected via a spring to the first one, and is oriented vertically with respect to the $z = 0$ plane, with its height being constrained to $z > 0$. Particles interact only with particles of the same type with a Lennard-Jones potential:

$$V^i(r) = \begin{cases} 4\epsilon\left[\left(\frac{\sigma}{r}\right)^{12} - \left(\frac{\sigma}{r}\right)^{6}\right] - \delta_1 & r \leq \sigma^i_{cut} \\ 0 & r > \sigma^i_{cut}, \end{cases} \tag{S1}$$

with $i = 1, 2$ the particle's type index. The cutoff distance is $\sigma^1_{cut} = \sigma_{min} = 2^{\frac{1}{6}}\sigma$ for type 1 particles, and is $\sigma^2_{cut} = 1.5\sigma$ for type 2 particle. Thus both types of particles are repulsive for distances $r < \sigma_{min}$, while type 2 particles attract each other if distances are between $\sigma_{min} < r < 1.5\sigma$. $\delta_1 = 4\epsilon\left[\left(\frac{\sigma}{\sigma^i_{cut}}\right)^{12} - \left(\frac{\sigma}{\sigma^i_{cut}}\right)^{6}\right]$ ensures that the potential is continuous at $\sigma^i_{cut}$.

Beads composing a dumbbell are connected by a quartic potential truncated in the center via a quadratic potential (Fig. S2), which acts only on the z-distance between dumbell beads:

$$V_{bond}(z) = \epsilon \begin{cases} d(z-c)^2 + e & r_1 \leq z \leq r_2 \\ a(z-c)^4 - b(z-c)^2 + h_q & otherwise \end{cases} \tag{S2}$$

The second term is the quartic potential, with $h_q$ the height of this potential barrier, $c$ the barrier center, and $2s$ the distance between two minima. We have that $a = \frac{h_q}{s^4}$ and $b = \frac{2h_q}{s^2}$. The first term of the potential represents the truncation part. We set $h_{trunc}$ as the value

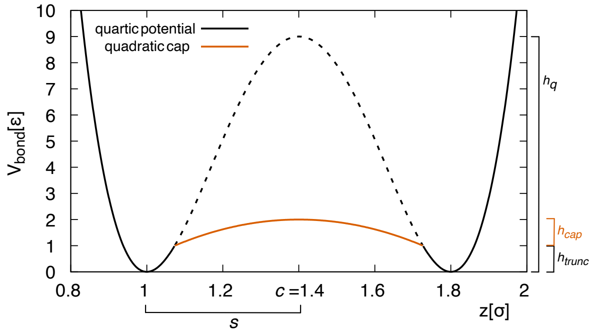


FIG. S2. Potential which connects two beads composing a dumbbell, and acting on the $z$ direction. It is composed by a quartic potential (black continuous line) and a quadratic central cap (red line).

where we want to truncate the quartic potential, and $h_{cap}$ as the additional height of the truncated cap. Thus, if $r_{1/2}$ are the values of the quartic potential at $h_{trunc}$, we have that $d = -\frac{h_{cap}}{(r_1-c)^2}$ and $e = h_{trunc} + h_{cap}$. We set for dumbbells $c = 1.4, s = 0.4, h_q = 9, h_{trunc} = 1, h_{cap} = 1$, such that the total potential height is $2\epsilon$. With this construction, the two potential wells are sufficiently narrow, while the barrier is sufficiently low to allow a fast transition between the two states.

A meaningful mapping can be established between the $z$ coordinate of the type 2 particle and two discrete spin states, with spin -1 for $z < c$ and spin +1 for $z \geq c$. Note that in Fig. 1-3 of the main text, we color the spin state via the formula $\frac{z-c}{s}$.

The $d_u$ and $d_s$ dumbbells, describing unsaturated and saturated lipids respectively, are biased in one spin state by considering a bond potential with an additional term:

$$V_{bond}^{bias}(z) = V_{bond}(z) + \frac{\epsilon\Delta}{2s}(z-c), \tag{S3}$$

with $\Delta$ the required energy distance shift between the two $V_{bond}$ minima. Here we use $\Delta = -2, 2$ in order to bias a dumbbell to have spin up ($d_s$) or down ($d_u$), respectively, and resulting in an energy difference between the two minima equal to $2\epsilon$.

The dumbbells oscillations around the axis $z$ are restricted through a harmonic potential. If $x$ and $y$ are the distances between dumbbell beads, we can define a harmonic potential which restrict these distances around zero:

$$V_{tilt} = \frac{1}{2}k(x^2 + y^2), \tag{S4}$$

with $k$ the harmonic constant. We used $k = 70$ for $d_u$ and $k = 10^4$ for $d_s$.

Channels consist of six dumbbells stacked together in a triangular lattice to form an hexagon (Fig. 3 of main text, and Fig S3), where each dumbbell is composed by type 1 (bottom) and type 2 (top) particles. These interact with other channels or lipids (we will refer from now on to $d_u$ and $d_s$ molecules as lipids) in the same way as described for lipids themselves: type 2 channel beads can be attracted by both type 2 lipid beads and other type 2 channel beads, while type 1 beads only feel excluded volume interactions with other type 1 beads of both channels and lipids. Each dumbbell of a channel has the same $V_{bond}$ potential, with $c = 1.4, s = 0.4, h_q = 9, h_{trunc} = 0.05, h_{cap} = 0.05$, such that the total potential height is $0.1\epsilon$, and is subjected to $V_{tilt}$ with $k = 10^4$. To ensure the channel structural integrity, each type 1 particle is connected to its neighbours via a harmonic potential $\frac{1}{2}k_1(r-r_0)^2$, with $k_1 = 495$ and $r_0 = \sigma$, with same curvature as $V_{bond}$ around one of the minima. Similarly, type 2 particles are connected to their type 2 neighbours with the same harmonic potential.

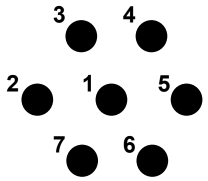


FIG. S3. 7-spin model representing the channel considered in the mesoscopic model. Numbers represent the spin labels.

Unlike lipids, channels are biased via an external force field $\mathbf{F}_p$ applied to type 2 particles and constructed to reproduce the membrane potential felt by ion channels:

$$\mathbf{F}_p = F_p\left(\frac{1}{1+e^{-100(z-1.1)}} - \frac{1}{1+e^{-100(z-1.7)}}\right)\mathbf{z} \tag{S5}$$

with $F_p$ the bias intensity and $\mathbf{z}$ the unit vector. The force is approximately constant and equal to $F_p$ for $1.1 < z < 1.7$ and zero otherwise.

Particles evolve via the Nose-Hoover equation of motion [4] at constant pressure $P = 0.2$, with the addition of a Langevin force term for each particle $i$:

$$\boldsymbol{F}_{lang} = -\gamma\dot{\boldsymbol{r}}_i + \sqrt{2k_BT\gamma}\boldsymbol{\eta}_i(t) \tag{S6}$$

where $T$ and $\gamma = 0.5$ are the temperature and friction, respectively, of the thermal bath in contact with the system, $m$ is the particle's mass, $k_B$ is the Boltzmann constant, $\boldsymbol{\eta}_i$ is an uncorrelated Gaussian noise with zero mean and unit variance. Note that the value of the pressure determines the PT melting curve of lipids, and thus the temperatures where the transition is located varying the elastic constant $k$. The chosen $P$ is optimal to obtain a separation between the melting temperatures observed for $k = 70, 10^4$. The force acting on the $z$-direction for type 1 particles is set to zero throughout the entire simulation, so that they move on the plane with $z = 0$. In the case of a single bare channel (without surrounding lipids), we considered instead a system at constant volume when taking measurements.

The potentials and the equation of motion described were implemented in a modified version of the LAMMPS software [5]. The reference units are the standard Lennard-Jones reduced units $m$, $\sigma$ and $\epsilon$, all set to unity, as well as the Boltzmann constant $k_B = 1$. Thus, the time units is $\tau_{LJ} = \sqrt{\frac{m\sigma^2}{\epsilon}}$. The timestep is set to $0.002\tau_{LJ}$.

The initial configuration is obtained by initializing lipids and channels in random positions inside a large box, with type 1 particles at z=0. The system was then evolved until it equilibrated at a given temperature. The typical equilibration time is around $3 \cdot 10^7$ timesteps. Afterwards, systems were evolved for a minimum of $10^8$ timesteps in order to sample data. We considered in the main text systems composed by 4096 or 9216 lipids, with the latter simulations used for the percolation analysis of Fig.3. We considered ratio of the number of channels to lipid equal to 0.005, 0.05, 0.075, 0.1, 0.15, 0.2.

The ordering of lipids is studied computing the hexatic order parameter on type 1 particles. In general, the hexatic order parameter is defined in a two-dimensional system for a particle $k$ as:

$$\psi_{6k} = \frac{1}{nn_k} \sum_{i=1}^{nn_k} e^{i6\theta_{ik}}, \tag{S7}$$

with $nn_k$ the number of nearest neighbors of particle $k$ within a distance of $1.5\sigma$ to the considered particle, and $\theta_{ik}$ the angle between the segment that connects $k$ with its neighbour $i$ and the $x$ axis. For beads regularly placed on the vertices of a triangular lattice, each site has six nearest-neighbours, all the angles are multiples of $2\pi/6$, and $|\psi_{6k}| = 1$. Small values of the absolute value of $\psi_{6k}$ indicate deviation from perfect orientational ordering.

Clustering of channels in Fig. 3 of the main text is performed using the DBSCAN algorithm. We clustered only the central type 1 particles of each channel, considering as clustering parameters $eps = 3.5$ and $minsampl = 2$, respectively the radius of the neighborhood with respect to some point and the minimum number of points in the neighborhood required to form a dense region.

The fit of the curves in Fig. 4b is performed using the analytical activation curve computed for the central pore spin (label 1 of Fig. S3) of an isolated system composed by seven spins arranged in a triangular lattice and forming an hexagon, Fig. S3. The Hill curve is obtained by computing the partition function $Z_u$ ($Z_d$) with $\sigma_1 = +1$ ($\sigma_1 = -1$), and then considering the free energy difference between the two fixed states $\sigma_1 = +1$ and $\sigma_1 = -1$, at fixed external field $h$:

$$W(h) = \frac{1}{\beta} \log\left(\frac{Z_u}{Z_d}\right) = \frac{1}{\beta} \log\left(\frac{P_{up}}{P_{down}}\right), \tag{S8}$$

with $P_{down} = 1 - P_{up}$, $\beta = \frac{1}{k_B T}$.

In order to compute $W(h)$, we started from the energy of the seven spin model:

$$H = -\mathcal{J}_0 \left[\sigma_1 \sum_{i=2}^{7} \sigma_i + \sum_{i=2}^{6} \sigma_i \sigma_{i+1} + \sigma_2 \sigma_7\right] - \alpha h \sum_{i=1}^{7} \sigma_i \tag{S9}$$

with $\mathcal{J}_0$ the interaction energy between spins, and the constant $\alpha$ which couples spins with the external field, similarly to a gating charge in an ion channel.

We then considered all possible states with fixed $\sigma_1 = +1$ or $\sigma_1 = -1$ and their associated energies, and obtained :

$$\begin{aligned} W(h) = \frac{1}{\beta} \log \Big[ & e^{\beta(12\mathcal{J}_0+7\alpha h)} + 6e^{\beta(6\mathcal{J}_0+5\alpha h)} + 6e^{\beta(4\mathcal{J}_0+3\alpha h)} + \\ & 9e^{\beta 3\alpha h} + 6e^{\beta(2\mathcal{J}_0+\alpha h)} + 12e^{\beta(-2\mathcal{J}_0+\alpha h)} + 2e^{\beta(-6\mathcal{J}_0+\alpha h)} + \\ & 6e^{-\beta\alpha h} + 9e^{\beta(-4\mathcal{J}_0-\alpha h)} + 6e^{\beta(-2\mathcal{J}_0-3\alpha h)} + e^{-\beta 5\alpha h} \Big] - \\ \frac{1}{\beta} \log \Big[ & e^{\beta(12\mathcal{J}_0-7\alpha h)} + 6e^{\beta(6\mathcal{J}_0-5\alpha h)} + 6e^{\beta(4\mathcal{J}_0-3\alpha h)} + \\ & 9e^{-\beta 3\alpha h} + 6e^{\beta(2\mathcal{J}_0-\alpha h)} + 12e^{\beta(-2\mathcal{J}_0-\alpha h)} + 2e^{\beta(-6\mathcal{J}_0-\alpha h)} + \\ & 6e^{\beta\alpha h} + 9e^{\beta(-4\mathcal{J}_0+\alpha h)} + 6e^{\beta(-2\mathcal{J}_0+3\alpha h)} + e^{\beta 5\alpha h} \Big]. \end{aligned} \tag{S10}$$

Note that the asymptotic function for $h \to \pm\infty$ is $W = \pm 12\mathcal{J}_0 + 2\alpha h$. Thus, one recovers that the difference in free energy of the two asymptotes is

$$\Delta W_0 = 24\mathcal{J}_0, \tag{S11}$$

providing a direct connection between $\Delta W_0$ and the coupling constant $\mathcal{J}_0$.

The equation $W(h)$ was used to fit the Hill plot function $k_B T \log(P_{up}/(1 - P_{up}))$ both for the bare channel, and the case of channels immersed in lipids where we considered an effective coupling constant $\mathcal{J}$ instead of $\mathcal{J}_0$. In all cases, we substituted in the equation $h$ with $F_p + sh$, where the constant $sh$ represents a possible horizontal shift in the function. $P_{up}$ was computed in simulations considering only the central pore dumbbell of the hexagonal channel.

We assumed that $\alpha$ is constant across the bare channel and the embedded channels, and fitted $\mathcal{J}_0$, $\mathcal{J}$ across all values of $T$ and $F_p$. In order to find the optimal value of $\alpha$, we plotted residual averages of total sum squared residuals (SSR) from all fits. The residual SSR has a minimum for $\alpha = 0.5637$ (Fig. S4). For each combination of ($T$, $F_p$), a 95% confidence interval was obtained from the parabolic plot of SSR fitted to $s$ versus $\mathcal{J}$ by applying a threshold SSR determined by the F-distribution [6].

Note that if we consider the Hill plots for the bare channel at different temperatures (Fig S5), all curves collapse, implying that the coupling constant for the bare channel, $\mathcal{J}_0$, is temperature independent, and consequently $\Delta W_0$ as well.

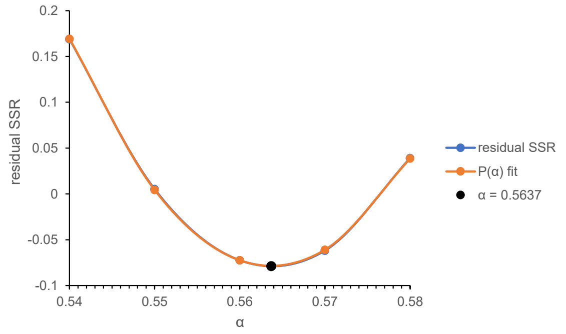


FIG. S4. Residual SSR relative to the average SSR over all conditions as a function of fixed $\alpha$. The fitting parabola, $P(\alpha)$, has a minimum at $\alpha = 0.5637$.

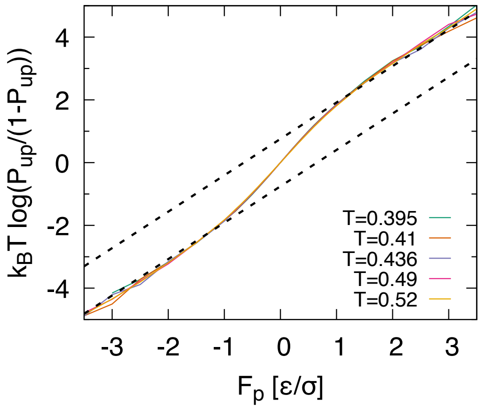


FIG. S5. Hill plot for a bare channel at different temperatures in the key. All curves collapse.

## III. MONTE CARLO SIMULATION OF LATTICE MODEL

For Monte Carlo simulations of a membrane system, we employed a $128 \times 128$ lattice with periodic boundary conditions to simulate clusters of tetrameric channels coupled to two lipid types, saturated and unsaturated. Channels consist of a 36-cell square boundary containing a central $2 \times 2$ cell pore surrounded by four $2 \times 2$ cell voltage sensors. The pore and voltage sensors gate between two "spin" states (closed/open and resting/activated) in a voltage-dependent manner. The remaining 16 cells of the channel domain are occupied by mobile lipid cells that exchange freely with bulk lipids. Spin flips in lipids are forbidden—therefore the starting 1:1 ratio between "unsaturated" and "saturated" species is maintained throughout the simulation (local Kawasaki dynamics). Channels and lipids diffuse freely, and channels can also rotate (Fig. 5b of the main text).

The kinetics of the lattice model are derived from the chemical master equation (CME). The CME is fundamental to ion channel modeling, where it is known as a "discrete-state Markov model" whose rate equations are encapsulated in a characteristic Q-matrix [7]. While for a $128 \times 128$ lattice system the Q-matrix is impossible to write down, much less solve, Monte Carlo methods can be used to simulate the time-trajectories of relatively large systems. Transition events are governed by first-order rate equations. The forward and backward rate constants of an event with intrinsic rate $\nu$ are expressed in a way that ensures detailed balance:

$$\text{forward rate} = \nu \exp\left(\frac{-(H_f - H_i)}{2k_BT}\right) \tag{S12}$$

$$\text{backward rate} = \nu \exp\left(\frac{-(H_i - H_f)}{2k_BT}\right), \tag{S13}$$

where $H_i$ and $H_f$ are the initial and final system energies for the forward process. The intrinsic rates for the lattice model described in the main text are $\nu_L = 10$ kHz (lipid translation), $\nu_C = 5$ kHz (channel translation), $\nu_R = 0.5$ kHz (channel rotation), $\nu_P = 2$ kHz (pore opening), and $\nu_J = 2$ kHz (voltage sensor activation). The kinetic parameters for channel activation ($\nu_P$ and $\nu_J$) were chosen so that the model channel activates within tens of milliseconds, as is typical for potassium channels [8, 9]. The translation rates for lipids and channels ($\nu_L$ and $\nu_C$) were chosen to be in line with reasonable diffusion rates in plasma membranes [10]. Translation rate constants are environment-dependent but 2D diffusion constants can be estimated for the neutral case $H_i = H_f$, from which we obtain $D = d_c^2\nu$, where $d_c$ is the cell length (about 0.8 nm for lipids). Based on this calculation lipid and channel diffusion rates are roughly 6.4 $\text{nm}^2$/ms and 3.2 $\text{nm}^2$/ms, respectively. The rotational rate ($\nu_R$) for channels is unknown, but a small rate (1/10 the rate of translational motion) was chosen to boost thermalization. Given that the rotational diffusion coefficient $D_R = (\pi/2)^2\nu_R$ is roughly related to the translational diffusion coefficient through $D_R = D/a_c^2$ [11], where $a_c$ is the effective channel radius, the choice of $\nu_R = 0.5$ kHz corresponds to an $a_c$ of 1.6 nm, which is the radius of gyration around the C4 symmetry axis of a K+ channel with known structure (Kv2.1, Ref. [12]).

The system free energy $H$ is the sum of nearest-neighbor coupling energies between lattice cells $(i, j)$ and the configuration energies of the channel gating particles $(k)$:

$$H = \sum_{i,j} W_{ij} + \sum_k W_k. \tag{S14}$$

Channel-lipid and channel-channel coupling consist of Ising-like interactions between "spin up" states {saturated; open; activated} and "spin down" states {unsaturated; closed; resting}. The coupling free energies for lipid-lipid ($W_{LL}$) and lipid-channel ($W_{LP}$, $W_{LJ}$) interactions ($P$ = pore; $J$ = voltage sensor) consist of

a penalty $\varepsilon = 22$ meV added to the system energy for each "opposite-spin" pair of cells. The value of the lipid-lipid coupling energy ($W_{LL}$) was chosen so that the nominal critical temperature for the lipid-only environment is $T_c = 16.7$ °C according to the Ising prescription $kT_c = \varepsilon/\ln(1+\sqrt{2})$, for which $k_BT_c = 25$ meV. The finite size of the system and the voltage-sensitive influence of ion channels softens and shifts critical-like behavior to a higher temperature. Because of Ising interactions between lipids, the membrane demixes in a temperature-dependent manner similar to the mesoscopic model.

Lipid-channel ($W_{LP}$ and $W_{LJ}$) interactions are experimentally about 1 $k_BT$ [13] and so these parameters were set equal to $W_{LL}$, which is roughly 1 $k_BT$. Channel-channel interactions are not well known but an attractive energy similar in scale to the other interactions (-25 meV) was assigned to $W_{JJ}$, the cell-cell interaction between voltage sensors from different channels.

The configuration free energies of the gating particles ($k = P, J$) are given by $W_k = E_k - S_kT - q_kV$. The particle energies are assigned to "spin-up" configurations, namely the open state of the pore ($P$) and the activated state of the voltage sensor ($J$). By assigning "spin-down" energies of gating particles to zero, the configuration energies may be viewed as transition energies of activation. We also assigned zero value to internal energy components ($E_k$), rendering the transition free energies purely entropic ($S_k$) except for the voltage-coupling term involving gating charge ($q_k$). A purely entropic transition is perhaps unrealistic but ensures that any temperature dependence experienced by the system can be attributed to coupling energies. Gating charges and transition entropies, as well as the coupling energies $W_C$ and $W_D$ (see next paragraph), were dictated by the shapes of typical Q-V and G-V curves measured in K+ channels, and BK channels in particular [14, 15]. The free energy parameters are: $S_P$ = -0.25 meV/K, $q_P$ = 1.0 $e_o$, $S_J$ = 0.3 meV/K, and $q_P = 2.25e_o$.

The partition function describing activation of the bare channel is given by:

$$Z = \left(C + J\right)^4 + P\left(1 + JD\right)^4, \tag{S15}$$

where $P$ and $J$ are equilibrium constants for pore and voltage-sensor activation and $C$, $D$ are allosteric factors that couple the pore and voltage sensors (P-J coupling). Each of the variables that make up $Z$ are Boltzmann factors of the form: $K = \exp(-W_k/k_BT)$, where the $W_k$ are the previously described configuration energies for gating particles, but for the coupling factors $C$, $D$ are assigned constant values $W_C$ = -10 meV, $W_D$ = -40 meV.

Experimentally relevant activation curves are the open probability $P_o$ and mean gating charge $\langle q\rangle$. The bare channel expressions of these curves (Fig S6) are easily obtained from $Z$ by evaluating the expressions $P_o = \partial \ln Z/\partial \ln P$ and $\langle q\rangle = k_BT\partial \ln Z/\partial V$ [16]. P-J coupling differs from symmetric Ising interactions in that the "up-up" and "down-down" interaction energies may be different. This "unbalanced" interaction scheme between pore and voltage sensor causes activation curves to "shift" with changes in voltage $V$. An Ising-like "balanced" interaction is realized when $C = D$. A thermodynamically relevant measure of $\langle q\rangle$ "shift" is the median voltage of activation $V_M = \int V(\partial Q/\partial V)dV$, where $Q$ is the normalized gating charge defined as $Q = \langle q\rangle/q_{max}$, and $q_{max}$ is the total charge [16, 17]. The median voltage of activation of the bare channel is given by the expression $V_M = -[(S_P + 4S_J)T + 4(W_C - W_D)]/q_{max}$. Changes in "balanced" P-J coupling, either directly or indirectly through interactions with lipids, will not shift $V_M$ but does steepen the Q-V curve. The maximum slope of the Q-V curve is a measure of cooperativity between voltage-gating domains. Another measure of cooperativity that selectively targets the interactions between pore and voltage sensors is the conductance Hill plot, defined as $W_{H[g]} = k_BT \ln P_o/(1 - P_o)$, taken as a function of $V$ [16, 18]. The vertical separation of the negative and positive asymptotic regions of the Hill plot is equal to the P-J coupling energy, which for the bare channel is $4(W_C + W_D)$.

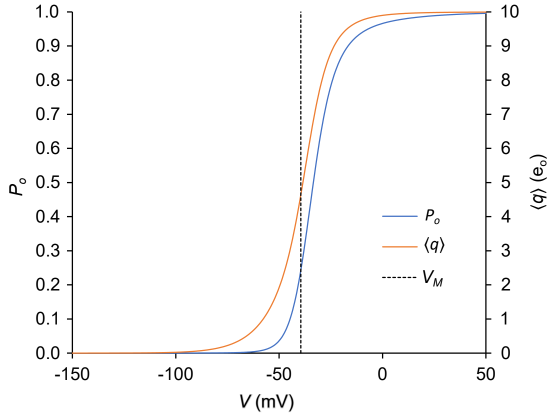


FIG. S6. $P_o$-$V$ and $\langle q\rangle$-$V$ curves of the bare channel at $T$ = 16.7 °C. The median voltage of activation is $V_M$ = -39.52 mV.

The kinetic Monte Carlo (KMC) method of Gillespie [19] was used to simulate trajectories of the bare channel as well as of 100 channels embedded in a 128×128 lipid-containing lattice. We employed two variations of KMC[20]. In method 1, after summing all transition rate constants accessible from a current configuration ($\sum\alpha$), one determines the time step $\tau$ from a uniform random variable $r_n$ through:

$$\tau = \frac{-\ln(1 - r_n)}{\sum \alpha} \tag{S16}$$

This is followed by a second step in which one accessible transition is chosen randomly using weighted probabilities in proportion to the transition rate constants. In method 2, one assigns a random time to each accessible transition using Eq. S16, except that the denominator

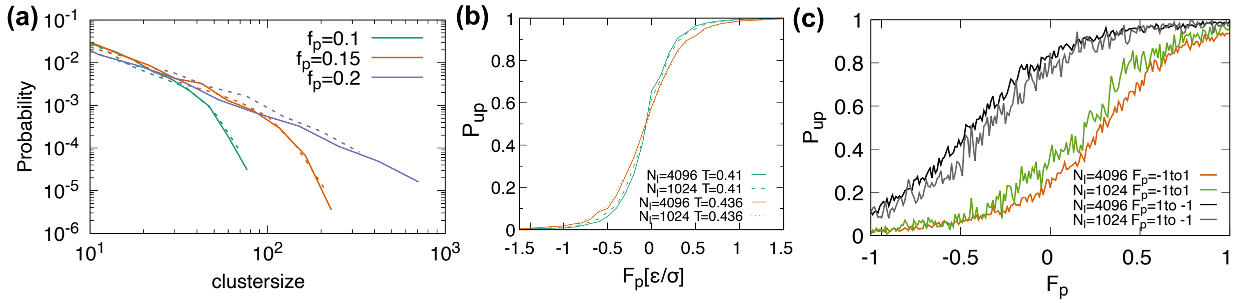


FIG. S7. (a) Comparison between cluster size distributions at $F_p = 0$ and $T = 0.436$ using a system with $N_l = 4096$ lipids (dashed lines) and $N_l = 9216$ lipids (continuum lines), with protein densities given in the key and for $F_p = 0$. The range of the distributions for the larger systems is wider. (b) Probability that the pore dumbbell of a channel is up as a function of the field $F_p$, comparing the case of $N_l = 4096$ lipids from Fig. 4d of the main text and the one for $N_l = 1024$ lipids, at $T = 0.41, 0.436$. We see a slight increase in cooperativity for $T = 0.41$. (c) Activation curves for $N_l = 4096$ lipids from Fig. 4d of the main text, compared with activation curves for $N_l = 1024$ lipids. These cases are for $T = 0.41$, $f_p = 0.05$ and a timing interval for the ramping of $\tau = 2 \cdot 10^4 \tau_{LJ}$. In the key is reported the direction of ramping of $F_p$. We see that is hysteresis is enhanced increasing the system size.

contains only the relevant rate constant. The transition with the smallest $\tau$ is allowed to proceed. Method 1 draws only two random numbers per iteration and is accordingly the more efficient of the two algorithms. Efficiency is further improved by keeping a running total of all accessible transitions and updating only those that are changed by the current transition.

But Eq. S16 only applies if rate constants are time-independent. In simulations with a ramping voltage protocol, voltage-dependent rate constants vary exponentially with time and at different rates depending on the gating charge. This requires method 2 to be used in conjunction with the following formula for $\tau$ [21]:

$$\tau = \frac{1}{\phi} \ln\left(1 - \frac{\phi}{\alpha} \ln(1 - r_n)\right) \tag{S17}$$

where $\phi = mq_k/k_BT$ and $m$ is the ramp speed in mV/ms. Eq. S17 reverts to Eq. S16 for constant voltage or zero gating charge. In practice, a hybrid approach for ramping protocols is used in which the collective sum of non-voltage-dependent (and therefore constant) transition rates is considered one rate for the purpose of method 2, and if chosen, a specific transition within the collective is chosen according to the second step of method 1. Conductance and gating charge trajectories were filtered to match the "experimental" sampling rate as previously described [22]. Slow-ramp data were sampled at 1 kHz and filtered using a Gaussian kernel with a cut-off frequency of 200 Hz.

## IV. FINITE SIZE EFFECTS

We show here possible effects arising from considering different system sizes. We expect in general that the system size imposes a cutoff on the maximum patch size encountered, and in turn the latter changes the characteristic time needed for channels to cross different patches. We thus expect that dynamical properties, rather than equilibrium ones, are more affected by finite size effects. Indeed, as shown below, hysteresis is more affected by system size, as it depends on the time required for channels to migrate from one patch to the other.

Starting from the mesoscopic model, we considered for the percolation transition a smaller system with $N_l = 4096$ lipids, compared with the one of 9216 lipids reported in Fig. 3a of the main text for $F_p = 0$. We found that the results produce the same distributions, but with a smaller range for smaller systems, see Fig. S7a. Regarding finite size effects for cooperativity, we compared curves reported in Fig.4a in the main text at $T = 0.41, 0.436$ obtained for a system of 4096, with ones obtained for 1024 lipids, see Fig. S7b. We do see a slight increase in cooperativity increasing the system size for the lower temperature. Regarding hysteresis, we compared a system with 1024 lipids with the one of 4096 lipids for curves in Fig. 4d of the main text, for $T = 0.41$ and $f_p = 0.05$, see Fig. S7c. We find that the field values for activations of half channels in the forward and backward ramping are significantly different for the two system sizes. We have for $N_l = 1024$ that $F^f_{1/2} = 0.207 \pm 0.024$ and $F^b_{1/2} = -0.304 \pm 0.024$, while for $N_l = 4096$ $F^f_{1/2} = 0.278 \pm 0.017$ and $F^b_{1/2} = -0.450 \pm 0.019$. Thus, hysteresis is enhanced increasing the system size.

With a similar approach to the mesoscopic model, we repeated the Hill, Q-V hysteresis, and Hurst analyses for systems of $64^2$ cells, compared to ones of $128^2$ cells considered in the main text, with same protein density. The results refer to values of Fig. 6 of the main text for $T = 30°C$. If we compare the Hill plot curves considering $64^2$ and $128^2$ cells, we find that $\Delta W/\Delta W_0$ changes from 1.65 to 1.7, thus a 2.8% increase. Regarding hysteresis, we find that $\Delta V_M$ changes from 10.5 to 12.2mV, with a 16.2% increase. Both results are consistent with observations of the mesoscopic model. We also do not

see significant changes in the Hurst exponent changing the system size, showing that long-term memory is unaffected.


[1] Daisuke Sato, Gonzalo Hernández-Hernández, Collin Matsumoto, Sendoa Tajada, Claudia M Moreno, Rose E Dixon, Samantha O'Dwyer, Manuel F Navedo, James S Trimmer, Colleen E Clancy, *et al.*, "A stochastic model of ion channel cluster formation in the plasma membrane," Journal of General Physiology **151**, 1116–1134 (2019).

[2] Antonio Coniglio and Annalisa Fierro, "Correlated percolation," in *Encyclopedia of Complexity and Systems Science*, edited by Robert A. Meyers (Springer New York, New York, NY, 2009) pp. 1596–1615.

[3] Aaron Clauset, Cosma Rohilla Shalizi, and M. E. J. Newman, "Power-law distributions in empirical data," SIAM Review **51**, 661–703 (2009).

[4] Wataru Shinoda, Motoyuki Shiga, and Masuhiro Mikami, "Rapid estimation of elastic constants by molecular dynamics simulation under constant stress," Physical Review B **69**, 134103 (2004).

[5] A. P. Thompson, H. M. Aktulga, R. Berger, D. S. Bolintineanu, W. M. Brown, P. S. Crozier, P. J. in 't Veld, A. Kohlmeyer, S. G. Moore, T. D. Nguyen, R. Shan, M. J. Stevens, J. Tranchida, C. Trott, and S. J. Plimpton, "LAMMPS - a flexible simulation tool for particle-based materials modeling at the atomic, meso, and continuum scales," Comp. Phys. Comm. **271**, 108171 (2022).

[6] Gerdi Kemmer and Sandro Keller, "Nonlinear least-squares data fitting in excel spreadsheets," Nature protocols **5**, 267–281 (2010).

[7] David Colquhoun and Alan G. Hawkes, *A Q-Matrix Cookbook* (Springer US, 1995) pp. 589–633.

[8] Enrico Stefani, Ligia Toro, Eduardo Perozo, and Francisco Bezanilla, "Gating of shaker K+ channels: I. Ionic and gating currents," Biophysical Journal **66**, 996–1010 (1994).

[9] William N Zagotta, Toshinori Hoshi, and Richard W Aldrich, "Shaker potassium channel gating. iii: Evaluation of kinetic models for activation." The Journal of general physiology **103**, 321–362 (1994).

[10] Eric N Senning and Sharona E Gordon, "Activity and Ca2+ regulate the mobility of TRPV1 channels in the plasma membrane of sensory neurons," Elife **4**, e03819 (2015).

[11] Reiner Peters and Richard J Cherry, "Lateral and rotational diffusion of bacteriorhodopsin in lipid bilayers: experimental test of the saffman-delbrück equations." Proceedings of the National Academy of Sciences **79**, 4317–4321 (1982).

[12] Ana I Fernández-Mariño, Xiao-Feng Tan, Chanhyung Bae, Kate Huffer, Jiansen Jiang, and Kenton J Swartz, "Inactivation of the Kv2.1 channel through electromechanical coupling," Nature , 1–8 (2023).

[13] Alison N Leonard and Edward Lyman, "Activation of G-protein-coupled receptors is thermodynamically linked to lipid solvation," Biophysical Journal **120**, 1777–1787 (2021).

[14] Frank T. Horrigan and Richard W Aldrich, "Coupling between voltage sensor activation, Ca2+ binding and channel opening in large conductance (BK) potassium channels." The Journal of General Physiology **120**, 267–305 (2002).

[15] Christopher Shelley, Xiaowei Niu, Yanyan Geng, and Karl L Magleby, "Coupling and cooperativity in voltage activation of a limited-state BK channel gating in saturating Ca2+," Journal of General Physiology **135**, 461–480 (2010).

[16] Daniel Sigg, "A linkage analysis toolkit for studying allosteric networks in ion channels," Journal of General Physiology **141**, 29–60 (2013).

[17] Sandipan Chowdhury and Baron Chanda, "Estimating the voltage-dependent free energy change of ion channels using the median voltage for activation," Journal of General Physiology **139**, 3–17 (2012).

[18] Sandipan Chowdhury and Baron Chanda, "Deconstructing thermodynamic parameters of a coupled system from site-specific observables," Proceedings of the National Academy of Sciences **107**, 18856–18861 (2010).

[19] Daniel T Gillespie, "Exact stochastic simulation of coupled chemical reactions," The journal of physical chemistry **81**, 2340–2361 (1977).

[20] Daniel T. Gillespie, "Stochastic simulation of chemical kinetics," Annual Review of Physical Chemistry **58**, 35–55 (2007).

[21] D Sigg and F Bezanilla, "Total charge movement per channel. the relation between gating charge displacement and the voltage sensitivity of activation." The Journal of general physiology **109**, 27–39 (1997).

[22] D. Sigg, H. Qian, and F. Bezanilla, "Kramers' diffusion theory applied to gating kinetics of voltage-dependent ion channels," Biophysical Journal **76** (1999).
